# Supplementary material for: Spatial Signatures of Electron Correlation in Least-Squares Tensor Hyper-Contraction
Source: arXiv:2409.14018 ancillary file (2024-09-21)
Supplement: Supplementary file 1 [file SI.pdf]

# Spatial Resolution of Electron Correlation in Least-Squares Tensor Hyper-contraction Methods: Supporting Information

Chao Yin, Sara Beth Becker, James H. Thorpe, and Devin A. Matthews*

*Department of Chemistry, Southern Methodist University, Dallas, TX 75275, USA*

E-mail: damatthews@smu.edu

# Optimized coordinates of all molecules in this study

All coordinates in Bohr.

Adenine

| | | | |
|---|---|---|---|
| N | -3.696893 | -0.847226 | 0.000000 |
| C | -2.544710 | -3.099028 | 0.000000 |
| N | -0.077204 | -3.591635 | 0.000000 |
| C | 1.292610 | -1.476396 | 0.000000 |
| C | 0.365721 | 0.990726 | -0.000001 |
| C | -2.278165 | 1.248107 | 0.000000 |
| N | 2.317740 | 2.729363 | -0.000001 |
| C | 4.366883 | 1.353121 | 0.000000 |
| N | 3.876499 | -1.204501 | 0.000000 |
| H | -3.790416 | -4.726518 | 0.000000 |
| H | 6.272436 | 2.077181 | 0.000001 |
| H | 5.143235 | -2.622218 | 0.000000 |
| N | -3.422561 | 3.525002 | -0.000001 |
| H | -5.318306 | 3.608207 | 0.000001 |
| H | -2.385182 | 5.112820 | 0.000000 |

AT-ST

| | | | |
|---|---|---|---|
| N | -1.101808 | -4.674066 | 0.612098 |
| C | -1.068384 | -4.754420 | -1.986965 |
| H | -2.438031 | -5.839712 | -3.034255 |
| N | 0.739647 | -3.390047 | -2.971792 |
| C | 1.955904 | -2.330858 | -0.914632 |
| C | 3.979882 | -0.623851 | -0.697024 |
| N | 5.205713 | 0.309534 | -2.732471 |
| H | 6.361490 | 1.788582 | -2.424700 |
| H | 4.302398 | 0.245794 | -4.406617 |
| N | 4.718108 | 0.081537 | 1.623019 |
| C | 3.469329 | -0.815121 | 3.626045 |
| H | 4.140511 | -0.164955 | 5.450791 |
| N | 1.496921 | -2.381691 | 3.667644 |
| C | 0.827865 | -3.097732 | 1.344812 |
| H | -2.421113 | -5.438204 | 1.748347 |
| N | -3.762294 | 1.267074 | 2.339831 |
| C | -1.855576 | 3.002082 | 2.651543 |
| H | -1.487372 | 3.545421 | 4.585989 |

| | | | |
|---|---|---|---|
| C | -0.523066 | 3.944937 | 0.702994 |
| C | 1.573027 | 5.813444 | 1.004265 |
| H | 3.379315 | 4.968176 | 0.481668 |
| H | 1.276215 | 7.447358 | -0.218091 |
| H | 1.707794 | 6.455700 | 2.956815 |
| C | -1.109949 | 3.026223 | -1.831850 |
| O | 0.005889 | 3.629171 | -3.750889 |
| N | -3.125378 | 1.312361 | -1.953157 |
| H | -3.483548 | 0.569968 | -3.675740 |
| C | -4.454237 | 0.278267 | 0.030167 |
| O | -6.058989 | -1.349367 | -0.208898 |
| H | -4.630480 | 0.503541 | 3.849947 |

AT-WC

| | | | |
|---|---|---|---|
| N | 1.742718 | -0.047103 | -0.708174 |
| C | 3.143008 | -0.051655 | 1.418374 |
| C | 5.788499 | -0.010397 | 1.130540 |
| C | 6.706998 | 0.024547 | -1.337594 |
| N | 5.338039 | 0.025195 | -3.460092 |
| C | 2.877370 | -0.010479 | -2.975903 |
| N | 7.745272 | 0.004135 | 2.861492 |
| C | 9.790363 | 0.045025 | 1.480515 |
| N | 9.289142 | 0.058939 | -1.076142 |
| N | 1.998139 | -0.109057 | 3.672597 |
| H | 1.603218 | -0.009918 | -4.581379 |
| H | 11.698586 | 0.066915 | 2.196725 |
| H | 10.548438 | 0.089224 | -2.500252 |
| H | 0.076922 | -0.055890 | 3.797604 |
| H | 3.068563 | -0.036168 | 5.238481 |
| N | -7.364680 | 0.010643 | -2.867664 |
| C | -8.682095 | 0.031495 | -0.636175 |
| C | -7.526402 | 0.035291 | 1.631355 |
| C | -4.767258 | 0.016170 | 1.659840 |
| N | -3.591954 | -0.008067 | -0.674963 |
| C | -4.747135 | -0.010209 | -3.000639 |
| C | -8.901665 | 0.057550 | 4.099087 |
| O | -3.512982 | 0.020785 | 3.614930 |
| O | -3.620127 | -0.027325 | -5.001211 |
| H | -8.266684 | 0.009841 | -4.542539 |
| H | -1.611396 | -0.029624 | -0.691133 |
| H | -10.718467 | 0.044954 | -0.821723 |
| H | -8.405435 | -1.594048 | 5.231673 |
| H | -8.383537 | 1.714185 | 5.214400 |

| | | | |
|---|---|---|---|
| H | -10.941449 | 0.069537 | 3.808068 |

Benzene

| | | | |
|---|---|---|---|
| C | 0.000000 | 2.628081 | 0.000000 |
| C | 0.000000 | -2.628081 | -0.000001 |
| C | -2.276234 | 1.314107 | 0.000000 |
| C | 2.276234 | 1.314107 | 0.000000 |
| C | -2.276234 | -1.314107 | 0.000000 |
| C | 2.276234 | -1.314107 | 0.000000 |
| H | 4.048219 | -2.337247 | 0.000000 |
| H | -4.048219 | -2.337247 | 0.000000 |
| H | 4.048219 | 2.337247 | 0.000000 |
| H | -4.048219 | 2.337247 | 0.000000 |
| H | 0.000000 | -4.674225 | 0.000000 |
| H | 0.000000 | 4.674225 | 0.000000 |

PFBA

| | | | |
|---|---|---|---|
| C | 4.203832 | 0.039333 | -0.421332 |
| O | 5.477764 | -1.191944 | -1.813303 |
| O | 4.793237 | 2.289402 | 0.557294 |
| H | 6.452598 | 2.766481 | -0.065826 |
| C | 1.569185 | -0.836796 | 0.537952 |
| F | 1.143892 | -3.183886 | -0.334173 |
| F | 1.587951 | -0.905618 | 3.094689 |
| C | -0.610760 | 0.925597 | -0.361645 |
| F | -0.526211 | 3.101822 | 0.949242 |
| F | -0.235817 | 1.442090 | -2.839004 |
| C | -3.323024 | -0.190845 | -0.067472 |
| F | -3.676432 | -1.022994 | 2.289226 |
| F | -3.704193 | -2.088673 | -1.675608 |
| F | -5.010247 | 1.623766 | -0.547049 |

Ph-criegee

| | | | |
|---|---|---|---|
| O | -5.001943 | 1.595444 | 0.000003 |
| O | -4.711441 | -0.962355 | 0.000000 |
| C | -2.522542 | -1.953277 | -0.000001 |
| H | -2.647157 | -4.000148 | -0.000003 |
| C | -0.085566 | -0.781776 | 0.000000 |
| C | 2.002830 | -2.438657 | 0.000000 |

| | | | |
|---|---|---|---|
| C | 0.344824 | 1.845975 | -0.000001 |
| C | 4.439964 | -1.508465 | 0.000001 |
| C | 2.804315 | 2.750281 | -0.000001 |
| C | 4.845045 | 1.095346 | 0.000000 |
| H | 1.681263 | -4.460325 | 0.000001 |
| H | -1.265914 | 3.089716 | -0.000001 |
| H | 6.027986 | -2.796370 | 0.000001 |
| H | 3.130260 | 4.769194 | -0.000001 |
| H | 6.755311 | 1.827786 | 0.000000 |

Thymine

| | | | |
|---|---|---|---|
| N | -2.099823 | 2.334163 | 0.000001 |
| C | -3.063491 | -0.095444 | 0.000000 |
| N | -1.198893 | -1.919271 | 0.000000 |
| C | 1.425691 | -1.563710 | 0.000001 |
| C | 2.235443 | 1.079922 | 0.000000 |
| C | 0.441046 | 2.880601 | 0.000000 |
| O | -5.307216 | -0.554694 | -0.000001 |
| O | 2.841314 | -3.371853 | 0.000001 |
| C | 5.009668 | 1.615816 | 0.000000 |
| H | -3.400032 | 3.722738 | 0.000000 |
| H | -1.808390 | -3.729348 | -0.000001 |
| H | 0.899230 | 4.873103 | 0.000001 |
| H | 5.372513 | 3.643687 | -0.000001 |
| H | 5.915566 | 0.779212 | 1.654105 |
| H | 5.915566 | 0.779211 | -1.654106 |

Hexane

| | | | |
|---|---|---|---|
| C | 2.617483 | 5.481609 | 0.000000 |
| C | -2.617483 | -5.481609 | 0.000000 |
| C | -0.000762 | 1.442072 | -0.000001 |
| C | 0.000761 | -1.442072 | -0.000001 |
| C | -2.644074 | -2.597098 | 0.000001 |
| C | 2.644074 | 2.597098 | 0.000001 |
| H | -4.529272 | -6.257495 | 0.000002 |
| H | 4.529273 | 6.257494 | 0.000002 |
| H | 1.640146 | 6.213614 | 1.665880 |
| H | 1.640150 | 6.213613 | -1.665883 |
| H | -1.640149 | -6.213613 | -1.665882 |
| H | -1.640146 | -6.213614 | 1.665881 |
| H | 3.683520 | 1.913427 | -1.653843 |

| | | | |
|---|---|---|---|
| H | 3.683518 | 1.913427 | 1.653845 |
| H | -3.683520 | -1.913427 | -1.653843 |
| H | -3.683518 | -1.913427 | 1.653845 |
| H | -1.042546 | 2.125978 | 1.654793 |
| H | -1.042545 | 2.125979 | -1.654795 |
| H | 1.042544 | -2.125979 | -1.654796 |
| H | 1.042546 | -2.125979 | 1.654792 |

Octane

| | | | |
|---|---|---|---|
| C | 0.004618 | 1.442347 | 0.000002 |
| C | -0.004619 | -1.442348 | 0.000002 |
| C | -2.636729 | 2.602043 | 0.000000 |
| C | 2.636728 | -2.602043 | 0.000001 |
| C | -2.629492 | 5.487413 | 0.000001 |
| C | 2.629492 | -5.487413 | 0.000001 |
| C | -5.279026 | 6.627383 | -0.000002 |
| C | 5.279027 | -6.627382 | -0.000002 |
| H | 1.049198 | 2.122028 | 1.654425 |
| H | 1.049201 | 2.122028 | -1.654420 |
| H | -1.049200 | -2.122029 | 1.654424 |
| H | -1.049200 | -2.122028 | -1.654421 |
| H | -3.682312 | 1.923072 | -1.654461 |
| H | -3.682314 | 1.923073 | 1.654460 |
| H | 3.682312 | -1.923073 | -1.654461 |
| H | 3.682314 | -1.923072 | 1.654460 |
| H | -1.584643 | 6.163681 | 1.653722 |
| H | -1.584640 | 6.163682 | -1.653719 |
| H | 1.584644 | -6.163681 | 1.653723 |
| H | 1.584640 | -6.163682 | -1.653718 |
| H | -5.216765 | 8.689859 | -0.000001 |
| H | -6.344686 | 6.030853 | -1.665791 |
| H | -6.344690 | 6.030852 | 1.665784 |
| H | 5.216766 | -8.689859 | -0.000002 |
| H | 6.344686 | -6.030852 | -1.665791 |
| H | 6.344690 | -6.030852 | 1.665784 |

Decane

| | | | |
|---|---|---|---|
| C | -0.004103 | 1.449705 | 0.000000 |
| C | 0.004103 | -1.449705 | 0.000000 |
| C | -2.666419 | 2.597952 | 0.000000 |
| C | 2.666419 | -2.597952 | 0.000000 |

| | | | |
|---|---|---|---|
| C | -2.683216 | 5.496920 | 0.000000 |
| C | 2.683216 | -5.496920 | 0.000000 |
| C | -5.346980 | 6.641401 | 0.000000 |
| C | 5.346980 | -6.641401 | 0.000000 |
| C | -5.346980 | 9.536879 | 0.000000 |
| C | 5.346980 | -9.536879 | 0.000000 |
| H | 1.040702 | 2.138769 | 1.660174 |
| H | 1.040702 | 2.138769 | -1.660174 |
| H | -1.040702 | -2.138769 | 1.660174 |
| H | -1.040702 | -2.138769 | -1.660174 |
| H | -3.710509 | 1.906947 | -1.659968 |
| H | -3.710509 | 1.906947 | 1.659968 |
| H | 3.710509 | -1.906947 | -1.659968 |
| H | 3.710509 | -1.906947 | 1.659968 |
| H | -1.640719 | 6.190482 | 1.660149 |
| H | -1.640719 | 6.190482 | -1.660149 |
| H | 1.640719 | -6.190482 | 1.660149 |
| H | 1.640719 | -6.190482 | -1.660149 |
| H | -6.388214 | 5.949398 | -1.659189 |
| H | -6.388214 | 5.949398 | 1.659189 |
| H | 6.388214 | -5.949398 | -1.659189 |
| H | 6.388214 | -5.949398 | 1.659189 |
| H | -7.274197 | 10.295884 | 0.000000 |
| H | -4.375404 | 10.285010 | 1.671642 |
| H | -4.375404 | 10.285010 | -1.671642 |
| H | 7.274197 | -10.295884 | 0.000000 |
| H | 4.375404 | -10.285010 | 1.671642 |
| H | 4.375404 | -10.285010 | -1.671642 |

# THC Analysis Scripts

This section contains descriptions of the scripts required to a) generate the THC data used in this work, and b) generate the plots and fits reported in this work based upon said data.

## Generating THC Data

**The results of the following steps are stored in the directories**

`SI/PartialEnergyAnalysis`

**and**

`SI/PairsofGridPointsAnalysis`

**after extraction of the compressed SI file for the reader's convenience, and can be used in later steps to regenerate the figures and fits of this manuscript without rerunning** CFOUR **or any of the scripts discussed below.**

The scripts required to reproduce the analysis in this manuscript are contained in the

`SI/THCpairpoints`

sub-directory, as well as a public GitHub repository located at : https://github.com/MatthewsResearchGroup/THCpairpoints . These scripts read various .dat files generated from the extract.py script after the successful completion of a CFOUR calculation. It should be noted that the THC-specific files can not be generated from the public version of CFOUR. Compressed .dat files used to generate the figures and data in this manuscript are provided in the GitHub repo. After extraction, .dat files for each given molecule/basis/wavefunction may be found in the following paths:

`data/grid/$molecule/*.dat`

The relevant file types are:

- fa.dat : diagonal of the virtual-virtual Fock Matrix
- fi.dat : diagonal of the occupied-occupied Fock Matrix
- t.dat : T2 amplitudes
- v.dat : abij electron repulsion integrals
- pvt.dat : pivots of the Cholesky grid pruning
- grid.dat : xyz coordinates and weight of a given grid point
- XI.dat : occupied-grid point collocation matrix
- XA.dat : virtual-grid point collocation matrix

**Gathering Base Data via** CFOUR

CFOUR calculations to generate data for these scripts must be run with Cartesian coordinates and in atomic units in order to be compatible with the Pair Point Analysis scripts below. Additionally, the scripts below only support RHF reference wavefunctions. The appropriate data files may be found on disk after the CFOUR calculation completes successfully and the "formatMolecule.sh" extraction script is run.

**Sub-directory Layout**

The partial energy analysis and pair point analysis scripts included in this repository expect a specific sub-directory layout for each molecule, where the name of each directory specifies the wavefunction and basis set for the given data, along with an additional sub-directory for THC grid data for any given basis set. The various options accepted by these scripts are given below:

- –molecule : any string
- –basis : any string

- –calc : { "MP2", "MP3", "CCSD" }

The path to the .dat files used in the following analysis then needs to adhere to the following pattern: $molecule/$basis/$calc for orbital data and $molecule/$basis/grid for grid data. For example, the orbital data for –molecule=thymine –basis=tz –calc=CCSD needs to be located in

```
thymine/tz/CCSD/*.dat
```

relative to the directory from which these scripts are called. The THC specific data for this same calculation would need to be located in

```
thymine/tz/grid/*.dat
```

If –calc=MP3 or –calc=MP2 then the calc directory should exist. For example, the orbital data for –molecule=thymine –basis=tz –calc=MP2 needs to be located in

```
thymine/tz/*.dat
```

and its THC data needs to be located in

```
thymine/tz/grid/*.dat
```

Likewise, if –basis=dz is used, the basis sub-directory should not exist. For example, the orbital data for –molecule=thymine –basis=dz –calc=CCSD needs to be located at

```
thymine/ccsd/*.dat
```

and the THC data at

```
thymine/grid/*.dat
```

These two rules compound, so if the options are –molecule=thymine –basis=dz –calc=MP2 the data needs to be located in

```
thymine/*.dat
```

and the THC data in

```
thymine/grid/*.dat
```

This description is also provided as a .pdf in the GitHub repository, and potential users are encouraged to defer to that description as these scripts may be modified or improved in future work.

### Partial Energy Analysis

The partial energy analysis programs are located in "partialGridEnergy" sub-directory. This program takes in the input described above and generates a series of THC approximations at increasing values of $\chi$ for the given contributions of $W_nT_2$ to the Coulomb and exchange correlation energies. These values are stored in a .csv file in in the path

```
$molecule/partialenergyanalysis_$method_$basis.csv
```

This script must be called at the top level of the specific sub-directory structure described in the previous subsection.

It should be noted that the Partial Energy Analysis depends upon the docopt.cpp and randutils libraries.

### Pair Point Analysis

The analysis of the pair point contributions to the THC approximations of $W_nT_2$ to the Coulomb and exchange correlation energies proceeds in several steps. The first step is to execute the "energyAnalysis" program, which accepts the –method input as described above and an additional parameter –npair that indicates the number of randomly selected pairs to be studied. This program must be called in the appropriate

```
$molecule/$basis
```

sub-directory for each method that will be analyzed. This program outputs

```
energyAnalysis_$method.csv
```

which contains the WSS and correlation energy contributions for the generated sets of pairs.

It should be noted that energyAnalysis depends upon the docopt.cpp and randutils libraries.

Once the full set of

```
$molecule/$basis/$method/energyAnalysis_$method.csv
```

files for a set of calculations have been generated and accumulated into a file called

```
$molecule/$basis/energyAnalysis.csv
```

the "make_ene_plot.py" script may be called to perform the bootstrapping and pair-point geometric analysis used to generate the correlation feature plots featured in the manuscript. This python script must be called from the top level directory of the pair-points analysis, and accepts only a fixed-format input:

```
python3 make_ene_plot.py $mol $basis $method $ftype $size
```

These options are summarized here:

- $mol : sub-directory name containing the data for a specific molecule.
- $basis : one of four strings, {adz, rtz, tz, dz }, which must also match the basis directory names in the sub-directory system.
- $method : a string that must match a method contained within $molecule/$basis/energyAnalysis.csv .
- $ftype : one of three strings, {all, no-cross, cross}. Analysis in this manuscript uses "all" exclusively.
- $size : an integer number of pairs of gridpoints, the same as those used –npair in energyAnalysis.

Upon completion, "make_ene_plot.py" will generate a large .csv file:

```
$molecule/$basis/bootstrapping_$mol_$basis_$method_$ftype.csv
```

along with a large number of figures contained within a new sub-directory called "pic". This .csv file is then used in the fitting and final set of plot generation.

**The results of the above steps are stored in the directories**

`SI/PartialEnergyAnalysis`

**and**

`SI/PairsofGridPointsAnalysis`

**for the reader's convenience, and can be used in the following steps to regenerate the figures and fits of this manuscript without rerunning** CFOUR **or any of the scripts discussed so far.**

## Using Pre-Generated Data

At this point, it is expected that the results of the partial energy fitting for all molecules, methods, and basis sets have been accumulated into one .csv file called "partialGridEnergy.csv". Likewise, the results of the pair point analysis for all molecules, methods, basis sets, and numbers of pairs of points, have been accumulated into

`Energy_Analysis_Bootstrapping_Merge.csv`

The versions of these files used in generating the plots and fits of this manuscript are located at

`SI/PartialEnergyAnalysis/partialGridEnergy.csv`

and

`SI/PairsofGridPointsAnalysis/Energy_Analysis_Bootstrapping_Merge.csv`

The following sections describe how to use the scripts located in SI/PairsofGridPointsAnalysis and SI/PartialEnergyAnalysis to generate the figures and fits reported in this work.

These scripts have been confirmed to work with the following package versions:

- Conda : 24.4.0
- Python: 3.10.13
- Pandas: 1.5.3
- MatPlotLib: 3.7.1
- NumPy: 1.24.3
- SciPy: 1.11.1
- SciKit-Learn: 1.3.0

We recommend that you execute these scripts within a conda environment with specific package versions. This may be created via the following shell commands:

```
conda create -n "THC-plotting"
conda init
\\close shell and reopen
conda activate "THC-plotting"
conda install pandas=1.5.3
conda install matplotlib=3.7.1
conda install numpy=1.24.3
conda install scipy=1.11.1
conda install scikit-learn=1.3.0
```

**Partial Energy Analysis Fits**

The script

SI/PartialEnergyAnalysis/PartialEnergyFitting.py

generates fits of THC approximations of $W_nT_2$ contributions to the Coulomb and exchange correlation energies as a function of $\chi$. The output of "partialGridEnergy" (described in the above section) for all species, wavefunctions, and basis sets needs to be contained within a single .csv file named "partialGridEnergy.csv". The script

SI/PartialEnergyAnalysis/PartialEnergyFitting.py

then generates a .csv file of the fit parameters, "PartialEnergyFittingParameters.csv", and a set of .png files that display the fits in a sub-directory called "PartialEnergyFitting" generated in the directory that the python script is called from.

### Partial Energy Analysis Method Comparison

The script

SI/PartialEnergyAnalysis/PartialEnergyComparsionMethods.py

generates comparisons for all the unique methods contained within "partialGridEnergy.csv" (same file as in the above subsection) for the THC approximations of $W_nT_2$ contributions to the Coulomb and exchange correlation energies. The output .png files are stored in a sub-directory called "PartialEnergyMethodsComparison" contained within the directory where "PartialEnergyComparsionMethods.py" is called from.

### Pair Points Fitting

The script

SI/PairsofGridPointsAnalysis/PairsofGridPointsFitting.py

generates the fit of the correlation feature used in the manuscript. It requires that

Energy_Analysis_Bootstrapping_Merge.csv

exists in the same directory from which it is called, and that this .csv file contains the accumulated results of the pair points analysis described above. Upon completion, this script will generate

`PairsofGridPointsFitting/Correlation_Feature_Gaussian_distribution_by_User.csv`

and

`PairsofGridPointsFitting/Correlation_Feature_t_coefficient_by_User.csv`

which contain the fits of the correlation feature to a Gaussian and Student's t-distribution, respectively.

### Pair Points Plotting

The script

`SI/PairsofGridPointsAnalysis/PairsofGridPointsPlotting.py`

is a python script that generates the plots of the correlation features used in the manuscript. It requires that

`Energy_Analysis_Bootstrapping_Merge.csv`

exists in the same directory from which it is called, and that this .csv file contains the accumulated results of the pair points analysis described above. Upon completion, this script will generate a new subdirectory called "PairsofGridPointsFigures", which in turn contains a significant number of figures sub-directories nested as

`PairsofGridPointsFigures/$molecule/$basis/$method`

In these directories there are a number of .png files that feature the plots listed below:

- EoverE : The ratio of the sum of exchange and Coulomb energy terms captured by pair grid points to the canonical correlation exchange and Coulomb energy terms, $\frac{\Delta E_x+\Delta E_c}{E_x+E_c}$

- WSS : the weighted subspace score introduced by the pair grid points
- ExoverEx : The ratio of exchange energy captured by pair grid points to the canonical correlation exchange energy, $\frac{\Delta E_x}{E_x}$
- EcoverEc : The ratio of Coulomb energy captured by pair grid points over the canonical correlation exchange energy, $\frac{\Delta E_c}{E_c}$
- ExoverE : The ratio of exchange energy captured by pair grid points to the total canonical correlation Coulomb energy, $\frac{\Delta E_x}{E_x+E_c}$
- EcoverE : The ratio of Coulomb energy captured by pair grid points to the total canonical correlation energy, $\frac{\Delta E_c}{E_x+E_c}$

WSS, EcoverE, and ExoverE are the types of plots used in the manuscript.
